# Supplementary material for: Providing Long-Term Participation Incentive in Participatory Sensing
Source: arXiv:1501.02480 source file (2016-02-24)
Supplement: Supplementary file 1 [file section-appendix.tex]

%!TEX root = main_participarory_sensing.tex
%SourceDoc main_participarory_sensing.tex

\appendix

\section{Appendix}

\subsection{Linear Programming Relaxation of Problem (\ref{problem:stochastic})}

By the linear programming relaxation, we relax $ \xn(\th) $ to real number in $ [0,1]$. Intuitively, the relaxed $ \xn(\th) \in[0,1] $ denotes the \emph{probability} that a user $n$ is selected as sensor under a particular information realization $\th$. 
Accordingly, we denote $\yi(\th) $ as the \emph{probability} that a grid $\ARi$ is sensed by at least one user under $\th$. That is, 
$$
\yi(\th)  = 1 - \Pi_{n=1}^N \big(1 - \xn(\th) \cdot  \zni(\th) \big). 
$$
Note that if $ \xn(\th) $ degrades to the integer number in $\{0,1\}$, then $\yi(\th) = \textsc{Step}(\sumN   \xn(\th) \cdot  \zni(\th) )  $, which is exactly same as that in the original problem (\ref{problem:stochastic}). 
Then, the relaxed social welfare maximization problem can be written as
\begin{equation}\label{problem:stochastic-relax}
\begin{aligned}
& \max_{ \bX }  \quad \intTH  \big( \V(\th) - \C(\th) \big) \cdot f(\th) \dd \th
\\
 & \mbox{s.t.} \txsty \quad \mbox{(a) } \xn(\th) \in \{0,1\},\quad \forall n\in\N, \forall \th\in\TH,
\\
& 
\txsty \quad ~~~ \mbox{(b) }  
\D_n \leq \d_n (\bxn) , \quad \forall n\in\N. 
%\\
%& 
%\txsty \quad \mbox{(c) }  
%\V (\th) = \sumI \yi(\th) \cdot  \wi(\th), \quad, \forall \th\in\TH,
%\\
%& 
%\txsty \quad \mbox{(d) } 
%\C(\th) = \sumN \xn(\th) \cdot  \cn(\th), \quad \forall \th\in\TH.
\end{aligned}
\end{equation}

\subsection{Proof for Lemma \ref{lemma:gap}}

We first notice that problem (\ref{problem:stochastic}) is {time-independent} but information-dependent.
Hence, the sensor selection in different slots with the same network  information must be identical, i.e., $\bx[t_1] = \bx[t_2]$ if
$\th[t_1] = \th[t_2]$. 
Then, by the law of large number, we have: 
\begin{enumerate}
\item
$ \frac{1}{T} \sumT   \xnt  \rightarrow \intTH \xn(\th)  f(\th) \dd \th $;
\item
$\frac{1}{T} \sumT \Vt \rightarrow \intTH   \V(\th)  f(\th) \dd \th $;
\item
$\frac{1}{T} \sumT \Ct \rightarrow \intTH   \C(\th)  f(\th) \dd \th$, if $T\rightarrow \infty$.
\end{enumerate}
This further implies that problems (\ref{problem:complete}) and (\ref{problem:stochastic}) are equivalent if $T\rightarrow \infty$, hence their solutions are also equivalent.

\subsection{Proof for Theorem \ref{theorem:2}}

To prove the optimality, we need to show that the \emph{expected} drift-plus-penalty $\mathbf{E} (\pnlt[t]) $ is well bounded under the proposed Policy \ref{algo:2}. 
It is notable that with a well-designed bound, we can prove the optimality directly by using the Lyapunov drift and optimization theorem in \cite{Neely}. 

%There is a non-negative constant $\omega \geq 0$ such that\footnote{Here, $\mathbf{E} (.)$ is the expectation operation with respect to $\th$.}
%$$
%\mathbf{E} (\pnlt[t]) \leq B - \omega  \sumN \quen^t - \lypV \cdot \VCso,
%$$ 
%where 
%%$\bar{\que}_n$ is the average backlog of $\quen$, and 
%$\VCso$ is the maximum social welfare benchmark with stochastic information (derived in Section \ref{sec:solution}).

%This upper-bound can be derived in the following way. 
Next we show how to find a desired bound for $\mathbf{E} (\pnlt[t]) $.  
Let $\bxlo[t]$ and $\VClo[t]\eq (\Vt - \Ct)|_{\bxlo[t]}$ denote the allocation vector and the achieved social welfare in slot $t$ using the Lyapunov-optimization based policy.
Let $\bxso[t]$ and $\VCso[t]\eq (\Vt - \Ct)|_{\bxso[t]}$ denote the allocation vector and the achieved social welfare in slot $t$ using the optimal allocation with stochastic information given in (\ref{problem:stochastic}).
We first have:
$$
\sumN \quen^{t} \cdot \xnlo[t] + \lypV \cdot \VClo[t]
\geq \sumN \quen^{t} \cdot \xnso[t] + \lypV \cdot \VCso[t] , 
$$
as $\xnlo[t]$ maximizes $\sumN \quen^{t} \cdot \xnt + \lypV \cdot \VC[t]$. 

Then, by (\ref{eq:penalty-bound}), we further have:
$$
\mathbf{E}(\pnlt[t]) 
 \leq B + \sumN \quen^{t} \cdot (\D_n - \mathbf{E} (\xnso[t])) - \lypV \cdot \mathbf{E} (\VCso[t]). 
$$

We further notice that $\mathbf{E} (\VCso[t]) = \VCso$, and $\mathbf{E} ( \xnso[t] ) = \dnso \geq \D_n$ by the constraint (b) in (\ref{problem:stochastic}). Hence, we can find an non-negative constant $\omega \eq \min_n(\dnso - \D_n)$, such that
$$
\mathbf{E}(\pnlt[t]) 
 \leq B -\omega \sumN  \quen^t - \lypV \cdot \VCso. 
$$
With this bound, we can prove  
the optimality directly by using the Lyapunov drift and optimization theorem in \cite{Neely}.

\subsection{Proof for Theorem \ref{lemma:truthfulness}}

We first show that each user $n$ has no incentive to report (bid) a cost \textbf{higher than} its true cost. 
There are 4 possible outcomes:
 
\noindent
(a) \{\emph{loss, loss}\}: user $n$ loses when bidding both truthfully and non-truthfully. It receives a zero payment in both strategies.~~~~ 

\noindent
(b) \{\emph{win, loss}\}: user $n$ wins (loses) when bidding truthfully (non-truthfully). It receives a smaller payment (i.e., zero) when bidding non-truthfully.
 
\noindent 
(c) \{\emph{loss, win}\}: user $n$ loses (wins) when bidding truthfully (non-truthfully). This is practically impossible, as a user losing with a lower cost will never win when submitting a higher cost. 

\noindent
(d) \{\emph{win, win}\}: user $n$ wins when bidding both truthfully and non-truthfully. We will show that user $n$ receives the same payment in both strategies.  
First, the third term and the last term in (\ref{eq:auction-pay}) are obviously identical in both strategies. 
Second, the first two terms in (\ref{eq:auction-pay}) are also identical due to the following assert: \emph{If an allocation vector $\bx^*$ maximizes the social welfare, then, excluding any user $n$ and removing the grids sensed by user $n$ (under $\bx^*$), the remaining vector $\bx_{-n}^*$ maximizes the social welfare in the remaining system.} 
 
We then show that each user $n$ has no incentive to report (bid) a cost \textbf{lower than} its true cost. 
Similarly, there are 4 possible outcomes:

\noindent
(a) \{\emph{loss, loss}\}: user $n$ loses when bidding both truthfully and non-truthfully. It receives a zero payment in both strategies.~~~~ 

\noindent
(b) \{\emph{win, loss}\}: user $n$ wins (losses) when bidding truthfully (non-truthfully). This is practically impossible, as a user winning at a higher cost will never lose when submitting a lower cost. 
 
\noindent 
(c) \{\emph{loss, win}\}: user $n$ loses (wins) when bidding truthfully (non-truthfully). 
Notice that there is a critical point such that user $n$ wins (loses) when its cost is lower (higher) than the critical point. 
In this case, user $n$'s true cost is higher than the critical point (as it loses when bidding truthfully). 
User $n$ wins only when it submits a cost lower than the critical point. 
We further notice that the above critical point is exactly the payment to user $n$. Hence, it receives a negative payment when bidding non-truthfully.  

\noindent
(d) \{\emph{win, win}\}: user $n$ wins when bidding both truthfully and non-truthfully. 
Similarly, we can show that user $n$ receives the same payment in both strategies.
